# Supplementary material for: Trackintel: An open-source Python library for human mobility analysis
Source: arXiv:2206.03593 ancillary file (2022-08-05)

# Trackintel case study

June 2, 2022

This notebook presents a case study to jointly analyse four different tracking datasets using [Trackintel](#). Three of the datasets that are used in this case study can not be published to protect the privacy of the participants. You can find an executable example notebook for trackintel here: [binder](#) and [code](#).

## Imports

```
[305]: import os, sys
from collections import defaultdict
import pickle
import datetime

import numpy as np
import pandas as pd
import geopandas as gpd
import matplotlib.pyplot as plt
import pytz
import json
import seaborn as sns
from shapely.geometry import Point, Polygon
from sqlalchemy import create_engine

from IPython.display import Image
from IPython.core.display import HTML

import trackintel as ti
from trackintel.analysis.tracking_quality import temporal_tracking_quality
from trackintel.analysis.modal_split import calculate_modal_split
from trackintel.visualization.modal_split import plot_modal_split
from trackintel.analysis.labelling import predict_transport_mode
plt.rcParams.update({"font.size": 15})
```

## Define paths & PostGIS connection

```
[42]: # output directory to save all outputs
out_path = "temp"
os.makedirs(out_path, exist_ok=True)
```

```

# Geolife data
path_to_geolife = "Geolife Trajectories 1.3/Data"

# for postgis
DBLOGIN_FILE_GC = "../../dblogin_commit.json"
DBLOGIN_FILE_yumuv = "../../dblogin_mielab.json"

with open(DBLOGIN_FILE_GC) as json_file:
    LOGIN_DATA_GC = json.load(json_file)

with open(DBLOGIN_FILE_yumuv) as json_file:
    LOGIN_DATA_YUMUV = json.load(json_file)

engine_gc = create_engine(
    "postgresql://{user}:{password}@{host}:{port}/{database}".format(
        **LOGIN_DATA_GC
    )
)
engine_yumuv = create_engine(
    "postgresql://{user}:{password}@{host}:{port}/{database}".format(
        **LOGIN_DATA_YUMUV
    )
)
engine_casestudy = create_engine(
    "postgresql://{user}:{password}@{host}:{port}/case_study_cache".format(
        **LOGIN_DATA_YUMUV
    )
)

CRS_WGS84 = "epsg:4326"

```

```

[30]: # short names of the four included datasets
studies = ["gc1", "gc2", "yumuv_graph_rep", "geolife"]

# Full names for plotting
study_mapping = {
    "gc1": "Green Class 1",
    "gc2": "Green Class 2",
    "yumuv_graph_rep": "Yumuv",
    "geolife": "Geolife",
}

```

## 1 Dataset loading and preprocessing

### 1.1 Datasets

We include the data from four tracking studies with two different tracking data types.

### 1.1.1 Green Class 1 & 2

The Green Class 1 & 2 studies were conducted in collaboration with the Swiss Federal Railway Systems (SBB) under the project name [SBB Green Class](#). In both studies, participants were given full access to all public transport in Switzerland. In addition, the participants from the first Green Class study (Green Class 1) received an electric vehicle and the ones from the second study (Green Class 2) an e-bike. Study participants were tracked with a GNSS-based application (app) that provides partially preprocessed data as staypoints and triplegs.

### 1.1.2 Geolife

The open-source [Geolife dataset](#) covers the movement of employees of Microsoft Research Asia. The dataset is from around 2012 and was still recorded with dedicated GPS-only trackers. As the study took place in an urban area the GPS was unreliable and there are many gaps in the dataset. However, Geolife is still one of the few publicly available tracking datasets.

### 1.1.3 Yumuv

The [yumuv](#) study investigated the impact of a [Mobility-as-a-Service app](#) that integrates shared e-scooters, e-bikes and public transport. In the yumuv study, participants were divided into control and treatment group and were tracked for three months using an app that already provides staypoints and triplegs.

### 1.1.4 Data import and preprocessing

One main advantage of trackintel is its ability to standardize the preprocessing of tracking data. For this, the different datasets have to be imported to geopandas dataframes that fulfill the requirements described on <https://trackintel.readthedocs.io/en/latest/modules/model.html>.

The trackintel data model consists of these different classes:

- positionfixes [pfs]: Raw GPS data.
- staypoints [sp]: Locations where a user spent a minimal time.
- triplegs [tpls]: Segments covered with one mode of transport.
- locations [loc]: Clustered staypoints.
- trips: Segments between consecutive activity staypoints (special staypoints that are not just waiting points).
- tours: Sequences of trips which start and end at the same location (if the column 'journey' is True, this location is home).

The Geolife dataset consists of only positionfixes while the other datasets are already processed to staypoints and triplegs by the tracking app. We will now import all datasets and combine them on the staypoints / triplegs level.

## 1.2 Import Geolife

Geolife is an important benchmark dataset. Trackintel therefore offers a dedicated function that reads in the Geolife dataset. The import function takes care of the required column format and names.

```
[24]: import trackintel
from trackintel.io.dataset_reader import read_geolife

pfs_geolife, _ = read_geolife(path_to_geolife, print_progress=True)
pfs_geolife[["user_id", "tracked_at", "geom", "elevation"]].head(3)
```

```
100%
182/182 [01:18<00:00, 2.32it/s]
```

```
[24]:
```

|         | user_id | tracked_at                | geom                       | elevation |
|---------|---------|---------------------------|----------------------------|-----------|
| id      |         |                           |                            |           |
| 7634985 | 0       | 2008-10-23 02:53:04+00:00 | POINT (116.31842 39.98470) | 149.9616  |
| 7634986 | 0       | 2008-10-23 02:53:10+00:00 | POINT (116.31845 39.98468) | 149.9616  |
| 7634987 | 0       | 2008-10-23 02:53:15+00:00 | POINT (116.31842 39.98469) | 149.9616  |

### 1.2.1 Geolife - Generate staypoints

We generate staypoints from the positionfixes and define all staypoints as relevant activities if they are longer than 25 minutes.

```
[26]: # extract staypoints
pfs_geolife, sp_geolife = pfs_geolife.as_positionfixes.generate_staypoints(
    gap_threshold=24 * 60,
    include_last=True,
    print_progress=True,
    dist_threshold=200,
    time_threshold=30,
    n_jobs=4,
)
sp_geolife["study"] = "Geolife"

# add activity flag to staypoints
sp_geolife = sp_geolife.as_staypoints.create_activity_flag(
    method="time_threshold", time_threshold=25
)
sp_geolife.head(3)
```

```
100%|
182/182 [02:30<00:00, 1.21it/s]
```

```
[26]:
```

|    | user_id | started_at                | finished_at               | elevation | geom                       | study   | is_activity |
|----|---------|---------------------------|---------------------------|-----------|----------------------------|---------|-------------|
| id |         |                           |                           |           |                            |         |             |
| 0  | 0       | 2008-10-23 03:03:45+00:00 | 2008-10-23 04:08:07+00:00 | 61.7220   | POINT (116.29917 39.98341) | Geolife | True        |
| 1  | 0       | 2008-10-23 04:32:52+00:00 | 2008-10-23 09:42:25+00:00 | 53.9496   | POINT (116.32451 39.99967) | Geolife | True        |
| 2  | 0       | 2008-10-23 11:10:42+00:00 | 2008-10-24 02:10:09+00:00 | 26.8224   | POINT (116.32105 40.00917) | Geolife | True        |

### 1.2.2 Geolife - Generate triplegs

```
[27]: %%time
pfs_geolife, tpls_geolife = pfs_geolife.as_positionfixes.generate_triplegs(
    sp_geolife, method="between_staypoints", gap_threshold=25
)
tpls_geolife["study"] = "Geolife"
tpls_geolife.head(3)
```

CPU times: user 6min 20s, sys: 38.7 s, total: 6min 58s

Wall time: 7min 31s

```
[27]:
```

|    | user_id | started_at                | finished_at               | geom                                              | study   |
|----|---------|---------------------------|---------------------------|---------------------------------------------------|---------|
| id |         |                           |                           |                                                   |         |
| 0  | 0       | 2008-10-23 02:53:04+00:00 | 2008-10-23 03:03:40+00:00 | LINESTRING (116.31842 39.98470, 116.31845 39.9... | Geolife |
| 1  | 0       | 2008-10-23 04:08:07+00:00 | 2008-10-23 04:32:47+00:00 | LINESTRING (116.28680 39.99578, 116.28545 39.9... | Geolife |
| 2  | 0       | 2008-10-23 09:42:25+00:00 | 2008-10-23 11:10:37+00:00 | LINESTRING (116.32016 40.00478, 116.32039 40.0... | Geolife |

## 1.3 Import Green Class 1 & 2

The green class datasets are stored in a postgres database and were already preprocessed to staypoints (static behavior) and triplegs (movement). To use them with trackintel, the data has to be adjusted to the data model. This means to create a geodataframe with the correct column names and timezone aware timestamps.

### 1.3.1 Green class - Staypoints

```
[35]: sp_gc = []
for study in ["gc1", "gc2"]:
    # download data
    sp_temp = gpd.GeoDataFrame.from_postgis(
        sql=f"""SELECT id, user_id, started_at, finished_at, geometry_raw,\
            purpose_validated FROM {study}.staypoints\
            where started_at <= finished_at""",
        con=engine_gc,
        geom_col="geometry_raw",
        index_col="id",
    )

    # transform to trackintel dataframe
    sp_temp = ti.io.read_staypoints_gpd(
        sp_temp,
        geom_col="geom",
        tz="UTC",
        crs=CRS_WGS84,
        mapper={"geometry_raw": "geom", "purpose_validated": "purpose"},
    )

    # green class specific definition of activities
```

```

sp_temp = sp_temp.as_staypoints.create_activity_flag(
    method="time_threshold", time_threshold=25
)
meaningful_purpose = ~sp_temp["purpose"].isin(["wait", "unknown"])
sp_temp.loc[meaningful_purpose, "is_activity"] = True

# keep study as attribute
sp_temp["study"] = study_mapping[study]

sp_gc.append(sp_temp)

# display output
print("Staypoints loaded successfully for GC1 and GC2.\
      Geometry not shown due to data protection.")
sp_temp.drop("geom", axis=1).head(3)

```

Staypoints loaded successfully for GC1 and GC2.      Geometry not shown due to data protection.

[35]:

|         | user_id                              | started_at                       | finished_at                      | purpose | is_activity | study         |
|---------|--------------------------------------|----------------------------------|----------------------------------|---------|-------------|---------------|
| id      |                                      |                                  |                                  |         |             |               |
| 3644805 | 2379ddac-f662-49a5-84be-6fae5c91a7e3 | 2017-09-17 12:57:18.869999+00:00 | 2017-09-17 15:55:03.536000+00:00 | leisure | True        | Green Class 2 |
| 3680485 | 2379ddac-f662-49a5-84be-6fae5c91a7e3 | 2017-09-28 14:41:47.967000+00:00 | 2017-09-28 16:11:56.680000+00:00 | errand  | True        | Green Class 2 |
| 3680768 | 2379ddac-f662-49a5-84be-6fae5c91a7e3 | 2017-09-28 16:22:26.680000+00:00 | 2017-09-28 16:32:23.947999+00:00 | unknown | False       | Green Class 2 |

### 1.3.2 Green class - Triplegs

[36]:

```

tpls_gc = []
for study in ["gc1", "gc2"]:
    # downlaod data using geopandas
    tpls_temp = gpd.GeoDataFrame.from_postgis(
        sql=f"""SELECT id, user_id, started_at, finished_at, mode_validated
                as mode, mode_validated as mode_detailed,
                geometry FROM {study}.triplegs where ST_IsValid(geometry)""",
        con=engine_gc,
        crs=CRS_WGS84,
        geom_col="geometry",
        index_col="id",
    )
    # transform to trackintel dataframe
    tpls_temp = ti.io.read_triplegs_gpd(
        tpls_temp,
        geom_col="geom",
        crs=CRS_WGS84,
        tz="UTC",
        mapper={"geometry": "geom"},
    )
    # keep study as attribute
    tpls_temp["study"] = study_mapping[study]

```

```

tpls_gc.append(tpls_temp)

# display output
print("Triplegs loaded successfully for GC1 and GC2.\
      Geometry not shown due to data protection.")
tpls_temp.drop("geom", axis=1).head(3)

```

Triplegs loaded successfully for GC1 and GC2.      Geometry not shown due to data protection.

[36]:

|         | user_id                              | started_at                       | finished_at                      | mode       | mode_detailed | study         |
|---------|--------------------------------------|----------------------------------|----------------------------------|------------|---------------|---------------|
| id      |                                      |                                  |                                  |            |               |               |
| 4350776 | c9aa08e2-1a5d-4d41-ae62-6110a9072b23 | 2018-05-21 11:52:32.192009+00:00 | 2018-05-21 11:57:26+00:00        | Mode::Ecar | Mode::Ecar    | Green Class 2 |
| 4350859 | c9aa08e2-1a5d-4d41-ae62-6110a9072b23 | 2018-05-22 06:38:32+00:00        | 2018-05-22 06:41:18+00:00        | Mode::Walk | Mode::Walk    | Green Class 2 |
| 3665724 | 75e13408-67ba-4c45-84ec-27b65de10680 | 2017-09-23 10:47:45.506017+00:00 | 2017-09-23 10:50:15.506000+00:00 | Mode::Walk | Mode::Walk    | Green Class 2 |

## 1.4 Import yumuv

The yumuv data is stored in a postgis database and it is already available as staypoints and triplegs. To use them with trackintel, the data has to be adjusted to the data model. This means to create a geodataframe with the correct column names and timezone aware timestamps. We furthermore conduct two additional preprocessing steps:

- We filter the tracking duration to the duration of the study which took place for most users from the 13th of July 2020 to the 15th of November 2020.
- We offset the user ids by a constant to be able to combine the data later with the other datasets without overlaps.

### 1.4.1 yumuv - Staypoints

[37]:

```

min_date = datetime.datetime(year=2020, month=7, day=13, tzinfo=pytz.utc)
max_date = datetime.datetime(year=2020, month=11, day=15, tzinfo=pytz.utc)

```

[43]:

```

sp_yumuv = ti.io.read_staypoints_postgis(
    "select id, user_fk, started_at, finished_at,\
    geometry from yumuv.staypoint",
    con=engine_yumuv,
    geom_col="geometry",
    crs=CRS_WGS84,
    index_col="id",
    tz="UTC",
    mapper={"user_fk": "user_id"},
)
sp_yumuv = sp_yumuv.rename({"geometry": "geom"}, axis=1).set_geometry("geom")

sp_yumuv["study"] = "Yumuv"

# yumuv specific definition of activities
sp_yumuv = sp_yumuv.as_staypoints.create_activity_flag(time_threshold=25)

```

```

# offset user id to avoid conflicts with other studies
sp_yumuv["user_id"] = sp_yumuv["user_id"] + 10000

# filter study duration
sp_date_flag = (sp_yumuv["started_at"] >= min_date) & (
    sp_yumuv["finished_at"] <= max_date)
sp_yumuv = sp_yumuv[sp_date_flag]

# display output
print("Staypoints loaded successfully for Yumuv.\
    Geometry not shown due to data protection.")
sp_yumuv.drop("geom", axis=1).head(3)

```

Staypoints loaded successfully for Yumuv. Geometry not shown due to data protection.

[43]:

|         | user_id | started_at                | finished_at               | study | is_activity |
|---------|---------|---------------------------|---------------------------|-------|-------------|
| id      |         |                           |                           |       |             |
| 6773023 | 15529   | 2020-08-28 17:32:47+00:00 | 2020-08-29 10:56:01+00:00 | Yumuv | True        |
| 6678616 | 15285   | 2020-08-22 12:23:03+00:00 | 2020-08-22 13:40:37+00:00 | Yumuv | True        |
| 6109237 | 15003   | 2020-07-13 12:20:46+00:00 | 2020-07-13 12:57:39+00:00 | Yumuv | True        |

#### 1.4.2 yumuv - Triplegs

```

[44]: tpls_yumuv = ti.io.postgis.read_triplegs_postgis(
    """select distinct on (id) id, user_fk, started_at,
    finished_at, track_mode_corrected,
    geometry FROM yumuv.tripleleg where ST_isvalid(geometry)""",
    con=engine_yumuv,
    geom_col="geometry",
    crs=CRS_WGS84,
    index_col="id",
    tz="UTC",
    mapper={"user_fk": "user_id"},
)
tpls_yumuv = tpls_yumuv.rename(
    {"geometry": "geom", "track_mode_corrected": "mode"}, axis=1
).set_geometry("geom")
tpls_yumuv["study"] = "Yumuv"

# offset user id
tpls_yumuv["user_id"] = tpls_yumuv["user_id"] + 10000

# filter study duration
tpls_date_flag = (tpls_yumuv["started_at"] >= min_date) & (
    tpls_yumuv["finished_at"] <= max_date

```



```
)
tpls_yumuv = tpls_yumuv[tpls_date_flag]

# display output
print("Triplegs loaded successfully for Yumuv.\
      Geometry not shown due to data protection.")
tpls_yumuv.drop("geom", axis=1).head(3)
```

Triplegs loaded successfully for Yumuv. Geometry not shown due to data protection.

```
[44]:
```

|         | user_id | started_at                | finished_at               | mode  | study |
|---------|---------|---------------------------|---------------------------|-------|-------|
| id      |         |                           |                           |       |       |
| 6097696 | 15018   | 2020-07-13 01:08:33+00:00 | 2020-07-13 01:11:53+00:00 | walk  | Yumuv |
| 6097774 | 14982   | 2020-07-13 03:42:00+00:00 | 2020-07-13 03:44:21+00:00 | walk  | Yumuv |
| 6097775 | 14982   | 2020-07-13 03:44:21+00:00 | 2020-07-13 03:49:35+00:00 | train | Yumuv |

## 1.5 Combine studies

All datasets are now loaded into the trackintel framework and all tracking data is represented as **staypoints** and **triplegs**. We can now represent all studies in a joint **staypoints** and a joint **triplegs** dataframe and process all studies jointly. To allow the joint analysis we have to perform the following steps:

- All staypoints and triplegs are combined in a single dataframe respectively.
- All user ids are represented as strings to have an id column with a single data type.
- We offset the ids of staypoints and triplegs so that they are unique across studies.

Furthermore we simplify the geometry of triplegs to reduce computation time.

### 1.5.1 All studies - combine staypoints

```
[45]: staypoints = pd.concat([sp_geolife] + sp_gc + [sp_yumuv])
      staypoints["user_id"] = staypoints["user_id"].astype(str)
```

### 1.5.2 All studies - combine triplegs

```
[46]: triplegs = pd.concat([tpls_geolife] + tpls_gc + [tpls_yumuv])
      triplegs["user_id"] = triplegs["user_id"].astype(str)
```

```
[47]: triplegs["geom"] = triplegs.simplify(1e-5, preserve_topology=False)
```

### 1.5.3 Offset ids to ensure unique IDs

```
[49]: for ix, study in enumerate(study_mapping.values()):
      sp_study_flag = staypoints["study"] == study
      tpls_study_flag = triplegs["study"] == study
```

```
staypoints.loc[sp_study_flag].index = staypoints.loc[
    sp_study_flag].index + ix * 10e7
triplelegs.loc[tpls_study_flag].index = triplelegs.loc[
    tpls_study_flag].index + ix * 10e7
```

```
[50]: # show a staypoint for each study (without user_id and geometry due to privacy)
staypoints[[
    "started_at", "finished_at", "study", "is_activity", "purpose"
]].groupby("study").head(1)
```

```
[50]:
```

|  | id      | started_at                       | finished_at                      | study         | is_activity | purpose |
|--|---------|----------------------------------|----------------------------------|---------------|-------------|---------|
|  | 0       | 2008-10-23 03:03:45+00:00        | 2008-10-23 04:08:07+00:00        | Geolife       | True        | None    |
|  | 3552473 | 2017-08-17 17:22:12+00:00        | 2017-08-17 18:04:00+00:00        | Green Class 2 | True        | home    |
|  | 6309557 | 2020-07-28 11:23:02+00:00        | 2020-07-28 13:22:05+00:00        | Yumuv         | True        | None    |
|  | 1321494 | 2016-11-23 07:27:13.687000+00:00 | 2016-11-23 07:51:43.687000+00:00 | Green Class 1 | True        | work    |

Finally we create a table that matches user ids to studies

```
[51]: user_study_matching = staypoints[["user_id", "study"]].drop_duplicates()
user_study_matching = user_study_matching.set_index("user_id")
```

## 1.6 Joint preprocessing - Trips, tours and locations

The representation of human mobility as `staypoints` and `triplelegs` is often not enough for a detailed analysis. We now use `trackintel` to process `staypoints` and `triplelegs` further into `trips`, `tours` and `locations`.

### 1.6.1 Create trips

```
[52]: staypoints, triplelegs, trips = ti.preprocessing.triplelegs.generate_trips(
    staypoints=staypoints, triplelegs=triplelegs,
    gap_threshold=15, add_geometry=True
)
```

```
[53]: trips = trips.join(user_study_matching, on="user_id")
```

```
[60]: trips.head(3)
```

```
[60]:
```

|  | id | user_id | started_at                | finished_at               | geom                                              | origin_staypoint_id | destination_staypoint_id | study   | tour_id | duration_s |
|--|----|---------|---------------------------|---------------------------|---------------------------------------------------|---------------------|--------------------------|---------|---------|------------|
|  | 0  | 0       | 2008-10-23 02:53:04+00:00 | 2008-10-23 03:03:40+00:00 | MULTIPOINT (116.31842 39.98470, 116.29917 39.9... | NaN                 | 0.0                      | Geolife | NaN     | 0.176667   |
|  | 1  | 0       | 2008-10-23 04:08:07+00:00 | 2008-10-23 04:32:47+00:00 | MULTIPOINT (116.29917 39.98341, 116.32451 39.9... | 0.0                 | 1.0                      | Geolife | NaN     | 0.411111   |
|  | 2  | 0       | 2008-10-23 09:42:25+00:00 | 2008-10-23 11:10:37+00:00 | MULTIPOINT (116.32451 39.99967, 116.32105 40.0... | 1.0                 | 2.0                      | Geolife | NaN     | 1.470000   |

### 1.6.2 Create locations

```
[54]: staypoints, locations = ti.preprocessing.generate_locations(
    staypoints,
    epsilon=30,
    num_samples=1,
```

```

distance_metric="haversine",
print_progress=True,
n_jobs=4,
)

```

```

100%
1172/1172 [00:13<00:00, 89.58it/s]

```

```
[55]: locations = locations.join(user_study_matching, on="user_id")
```

```
[59]: locations.head(3)
```

```
[59]:
```

|    | user_id | center                     | extent                                            | study   |
|----|---------|----------------------------|---------------------------------------------------|---------|
| id |         |                            |                                                   |         |
| 0  | 0       | POINT (116.29917 39.98341) | POLYGON ((116.29952 39.98341, 116.29952 39.983... | Geolife |
| 1  | 0       | POINT (116.32446 39.99988) | POLYGON ((116.32439 39.99965, 116.32419 39.999... | Geolife |
| 2  | 0       | POINT (116.32089 40.00921) | POLYGON ((116.32155 40.00895, 116.32022 40.009... | Geolife |

### 1.6.3 Create tours

```
[60]: trips, tours = ti.preprocessing.generate_tours(
      trips, staypoints=staypoints, print_progress=True
)
tours["started_at"] = pd.to_datetime(tours["started_at"])
tours["finished_at"] = pd.to_datetime(tours["finished_at"])

```

```
[57]: tours = tours.join(user_study_matching, on="user_id")
```

```
[58]: tours.head(3)
```

```
[58]:
```

|    | user_id | started_at                | finished_at               | origin_staypoint_id | destination_staypoint_id | trips            | location_id | study   | nb_hops |
|----|---------|---------------------------|---------------------------|---------------------|--------------------------|------------------|-------------|---------|---------|
| id |         |                           |                           |                     |                          |                  |             |         |         |
| 0  | 0       | 2008-11-13 13:53:46+00:00 | 2008-11-14 01:59:25+00:00 | 19.0                | 21.0                     | [21, 22]         | 1           | Geolife | 2       |
| 1  | 0       | 2008-11-14 11:17:04+00:00 | 2008-11-14 11:18:34+00:00 | 25.0                | 26.0                     | [26]             | 2           | Geolife | 1       |
| 2  | 0       | 2008-11-14 07:03:48+00:00 | 2008-11-14 16:29:15+00:00 | 23.0                | 27.0                     | [24, 25, 26, 27] | 11          | Geolife | 4       |

## 2 Dataset comparison

### 2.1 Simple Statistics

Number of users, number of trips, number of trips by user, etc

```
[61]: overview_df = pd.DataFrame(index=study_mapping.values())

overview_df["nr_user"] = staypoints.groupby(by=["study"]).agg(
    {"user_id": "nunique"}
)
nr_user = overview_df["nr_user"]

```

```

# nb staypooints
overview_df["nr_sp"] = staypoints.groupby(by=["study"]).size()
overview_df["nr_staypoints_per_user"] = overview_df["nr_sp"] / nr_user

# nb triplegs
overview_df["nr_tpls"] = triplegs.groupby(by=["study"]).size()
overview_df["nr_triplegs_per_user"] = overview_df["nr_tpls"] / nr_user

# nb trips
overview_df["nr_trips"] = trips.groupby(by=["study"]).size()
overview_df["nr_trips_per_user"] = overview_df["nr_trips"] / nr_user

# nb locations
overview_df["nr_loc"] = locations.groupby(by=["study"]).size()
overview_df["nr_locations_per_user"] = overview_df["nr_loc"] / nr_user

# nb tours
overview_df["nr_tours"] = tours.groupby(by=["study"]).size()
overview_df["nr_tours_per_user"] = overview_df["nr_tours"] / nr_user

```

```
[62]: overview_df
```

```
[62]:
```

|               | nr_user | nr_sp  | nr_staypoints_per_user | nr_tpls | nr_triplegs_per_user | nr_trips | nr_trips_per_user |
|---------------|---------|--------|------------------------|---------|----------------------|----------|-------------------|
| Green Class 1 | 139     | 326925 | 2351.978417            | 465189  | 3346.683453          | 241827   | 1739.762590       |
| Green Class 2 | 50      | 87884  | 1757.680000            | 128618  | 2572.360000          | 61421    | 1228.420000       |
| Yumuv         | 806     | 326271 | 404.802730             | 502292  | 623.191067           | 199735   | 247.810174        |

  

|               | nr_loc | nr_locations_per_user | nr_tours | nr_tours_per_user |
|---------------|--------|-----------------------|----------|-------------------|
| Green Class 1 | 104497 | 751.776978            | 94977    | 683.287770        |
| Green Class 2 | 35715  | 714.300000            | 22709    | 454.180000        |
| Yumuv         | 127320 | 157.965261            | 83019    | 103.001241        |

## 2.2 Trip characteristics

- How many trips comprise one tour on average? How many triplegs comprise a trip?
- What is the average trip duration / distance?

### 2.2.1 Number of hops in tours

```
[63]: tours["nb_hops"] = tours["trips"].apply(lambda x: len(x))
overview_df["avg_hops_tours"] = tours.groupby("study")["nb_hops"].mean()
```

```
[64]: overview_df["avg_hops_tours"]
```

```
[64]: Green Class 1    2.725197
Green Class 2    2.656656
Yumuv           2.112806
Geolife          2.373469
Name: avg_hops_tours, dtype: float64
```

### 2.2.2 Trip duration

```
[65]: trips["duration_s"] = (  
        trips["finished_at"] - trips["started_at"]  
    ).dt.total_seconds() / 3600
```

```
[66]: overview_df[["mean_trip_dur", "std_trip_dur"]] = trips.groupby(  
        "study"  
    )["duration_s"].aggregate(["mean", "std"])
```

```
[67]: overview_df[["mean_trip_dur", "std_trip_dur"]]
```

```
[67]:
```

|               | mean_trip_dur | std_trip_dur |
|---------------|---------------|--------------|
| Green Class 1 | 0.522175      | 0.731360     |
| Green Class 2 | 0.513715      | 0.753746     |
| Yumuv         | 0.681057      | 0.911373     |
| Geolife       | 0.640133      | 0.935874     |

### 2.2.3 Overall tracking period

```
[68]: min_max_times_by_user = trips.groupby(["study", "user_id"]).aggregate(  
        {"started_at": "min", "finished_at": "max"}  
    )  
    duration_by_user = (  
        min_max_times_by_user[  
            "finished_at"  
        ] - min_max_times_by_user["started_at"]  
    ).dt.total_seconds() / (3600 * 24)  
  
    overview_df[  
        ["mean_tracking_period", "std_tracking_period"]  
    ] = duration_by_user.groupby("study").aggregate(["mean", "std"])
```

```
[69]: overview_df[["mean_tracking_period", "std_tracking_period"]]
```

```
[69]:
```

|               | mean_tracking_period | std_tracking_period |
|---------------|----------------------|---------------------|
| Green Class 1 | 401.639038           | 59.289224           |
| Green Class 2 | 314.203054           | 76.458555           |
| Yumuv         | 87.393827            | 38.954972           |
| Geolife       | 193.216082           | 443.133363          |

### 2.2.4 Number of trips per day per user

```
[70]: # average trips per day over full tracking period  
    nr_trips_per_user_per_day = (trips.groupby(  
        ["study", "user_id"]  
    ).size() / duration_by_user).groupby("study").mean()  
    overview_df["nr_trips_per_user_per_day"] = nr_trips_per_user_per_day
```

```
[71]: overview_df["nr_trips_per_user_per_day"]
```

```
[71]: Green Class 1      4.319424
      Green Class 2      3.797688
      Yumuv             3.131575
      Geolife            1.701115
      Name: nr_trips_per_user_per_day, dtype: float64
```

## 2.2.5 Trip distance

```
[72]: # compute length
      triplegs["length_in_m"] = ti.geogr.distances.calculate_haversine_length(
          triplegs
      )
```

```
[73]: # aggregate lengths
      metrics_per_trip = triplegs.groupby(["study", "trip_id"]).agg(
          {"trip_id": "count", "length_in_m": "sum"}
      )

      # add to results
      overview_df[
          ["nr_legs_per_trip", "avg_trip_length", "std_trip_length"]
      ] = metrics_per_trip.groupby("study").agg(
          {"trip_id": "mean", "length_in_m": ["mean", "std"]}
      )
```

```
[74]: overview_df[["nr_legs_per_trip", "avg_trip_length", "std_trip_length"]]
```

```
[74]:
```

|               | nr_legs_per_trip | avg_trip_length | std_trip_length |
|---------------|------------------|-----------------|-----------------|
| Green Class 1 | 1.923644         | 27353.308940    | 4.786795e+05    |
| Green Class 2 | 2.094039         | 33656.574834    | 5.681591e+05    |
| Yumuv         | 2.514616         | 16883.392910    | 1.004259e+05    |
| Geolife       | 1.000000         | 36091.470622    | 3.163541e+06    |

## 2.2.6 Tracking quality (temporal coverage)

```
[75]: triplegs_staypoints = pd.concat([triplegs, staypoints])
```

```
[76]: tracking_quality_by_user_study = triplegs_staypoints.groupby(
      "study"
  ).apply(temporal_tracking_quality)
      overview_df[
          ["mean_tracking_quality", "std_tracking_quality"]
      ] = tracking_quality_by_user_study.groupby("study")["quality"].agg(
          ["mean", "std"]
      )
```

```
[77]: overview_df[["mean_tracking_quality", "std_tracking_quality"]]
```

```
[77]:
```

|               | mean_tracking_quality | std_tracking_quality |
|---------------|-----------------------|----------------------|
| Green Class 1 | 0.846193              | 0.170515             |
| Green Class 2 | 0.753790              | 0.237544             |
| Yumuv         | 0.766790              | 0.231347             |
| Geolife       | 0.397451              | 0.317477             |

## 2.3 Finalize results in two tables

### 2.3.1 Present simple dataset statistics as nice table

```
[78]: # basic info
overview_df.fillna(0, inplace=True)
df_basic = overview_df[
    [
        "nr_user",
        "mean_tracking_period",
        "std_tracking_period",
        "nr_loc",
        "nr_sp",
        "nr_tpls",
        "nr_trips",
        "nr_tours",
    ]
].astype(int)
```

```
[79]: # format mean tracking period and its std nicely
df_basic["Tracking period (std)"] = df_basic.apply(
    lambda x: f"{x['mean_tracking_period']} ({x['std_tracking_period']})",
    axis=1
)
df_basic.drop(
    columns=["mean_tracking_period", "std_tracking_period"], inplace=True
)
```

```
[80]: # set column values for data type and tracking technology
df_basic.loc[
    ["Green Class 1", "Green Class 2", "Yumuv"], "Input"
] = "Staypoints, Triplegs"
df_basic.loc["Geolife", "Input"] = "Positionfixes"

df_basic.loc[
    ["Green Class 1", "Green Class 2", "Yumuv"], "Study type"
] = "GNSS (app)"
df_basic.loc["Geolife", "Study type"] = "GPS tracker"
```

```
[81]: # rename columns and index
df_basic = df_basic.rename(
    columns={
        "nr_user": "Users",
        "nr_loc": "Locations",
        "nr_sp": "Staypoints",
        "nr_tpls": "Triplegs",
        "nr_trips": "Trips",
        "nr_tours": "Tours",
    },
    index=study_mapping,
)

[82]: # select the columns in the right order
df_basic = df_basic[
    [
        "Users",
        "Tracking period (std)",
        "Input",
        "Study type",
        "Locations",
        "Staypoints",
        "Triplegs",
        "Trips",
        "Tours",
    ]
]

df_basic
```

[82]:

|               | Users | Tracking period (std) | Input                | Study type  |
|---------------|-------|-----------------------|----------------------|-------------|
| Green Class 1 | 139   | 401 (59)              | Staypoints, Triplegs | GNSS (app)  |
| Green Class 2 | 50    | 314 (76)              | Staypoints, Triplegs | GNSS (app)  |
| Yumuv         | 806   | 87 (38)               | Staypoints, Triplegs | GNSS (app)  |
| Geolife       | 177   | 193 (443)             | Positionfixes        | GPS tracker |

  

|               | Locations | Staypoints | Triplegs | Trips  | Tours |
|---------------|-----------|------------|----------|--------|-------|
| Green Class 1 | 104497    | 326925     | 465189   | 241827 | 94977 |
| Green Class 2 | 35715     | 87884      | 128618   | 61421  | 22709 |
| Yumuv         | 127320    | 326271     | 502292   | 199735 | 83019 |
| Geolife       | 13575     | 28877      | 30205    | 30199  | 7184  |



### 2.3.2 Present the trip statistics as nice table

```
[268]: # Analysis table
df_detailed = overview_df[
    [
        "nr_trips_per_user_per_day",
        "mean_trip_dur",
        "std_trip_dur",
        "avg_hops_tours",
        "nr_legs_per_trip",
        "avg_trip_length",
        "std_trip_length",
        "mean_tracking_quality",
        "std_tracking_quality",
    ]
]

df_detailed = df_detailed.round(2)

[271]: # # format mean and its std nicely in a single cell
to_km = lambda x: (x/1000).round(1)
df_detailed["Trip distance (std)"] = df_detailed.apply(
    lambda x: f"{to_km(x['avg_trip_length'])} ({to_km(x['std_trip_length'])})",
    axis=1
)
df_detailed["Trip duration (std)"] = df_detailed.apply(
    lambda x: f"{x['mean_trip_dur']} ({x['std_trip_dur']})", axis=1
)
df_detailed["Tracking quality (std)"] = df_detailed.apply(
    lambda x: f"{x['mean_tracking_quality']} ({x['std_tracking_quality']})",
    axis=1
)

[272]: df_detailed = df_detailed.rename(
    columns={
        "nr_trips_per_user_per_day": "Trips per day",
        "avg_hops_tours": "Trips per tour",
        "nr_legs_per_trip": "Legs per trip",
    }
)
df_detailed.drop(
    [
        "avg_trip_length",
        "std_trip_length",
        "mean_tracking_quality",
        "std_tracking_quality",
        "mean_trip_dur",
    ]
)
```

```

        "std_trip_dur",
    ],
    axis=1,
    inplace=True,
)

df_detailed

```

[272]:

|               | Trips per day | Trips per tour | Legs per trip | Trip distance (std) | Trip duration (std) | Tracking quality (std) |
|---------------|---------------|----------------|---------------|---------------------|---------------------|------------------------|
| Green Class 1 | 4.32          | 2.73           | 1.92          | 27.4 (478.7)        | 0.52 (0.73)         | 0.85 (0.17)            |
| Green Class 2 | 3.80          | 2.66           | 2.09          | 33.7 (568.2)        | 0.51 (0.75)         | 0.75 (0.24)            |
| Yumuv         | 3.13          | 2.11           | 2.51          | 16.9 (100.4)        | 0.68 (0.91)         | 0.77 (0.23)            |
| Geolife       | 1.70          | 2.37           | 1.00          | 36.1 (3163.5)       | 0.64 (0.94)         | 0.4 (0.32)             |

## 2.4 KDE plot for user tracking quality distribution

We have calculated the temporal coverage of the tracking data as an indicator for the tracking quality. The indicator was calculated for every individual user. We'll now plot the distribution over users for each dataset.

[90]:

```

# pivot to match seaborn requirements
tracking_quality_df = tracking_quality_by_user_study.reset_index(
    level=0
).pivot(columns="study", values="quality")

```

[230]:

```

fig, ax = plt.subplots(figsize=(9, 5))
g = sns.kdeplot(
    data=tracking_quality_df,
    fill=True,
    alpha=0.3,
    legend=True,
    common_grid=True,
    common_norm=False,
    ax=ax,
)

plt.ylabel("Density (users)", fontsize=20)
plt.xlabel("Tracking quality", fontsize=20)
sns.move_legend(g, "upper left")
plt.xlim(0, 1)
plt.savefig(os.path.join(out_path, "tracking_quality_kde.pdf"))
plt.show()

```

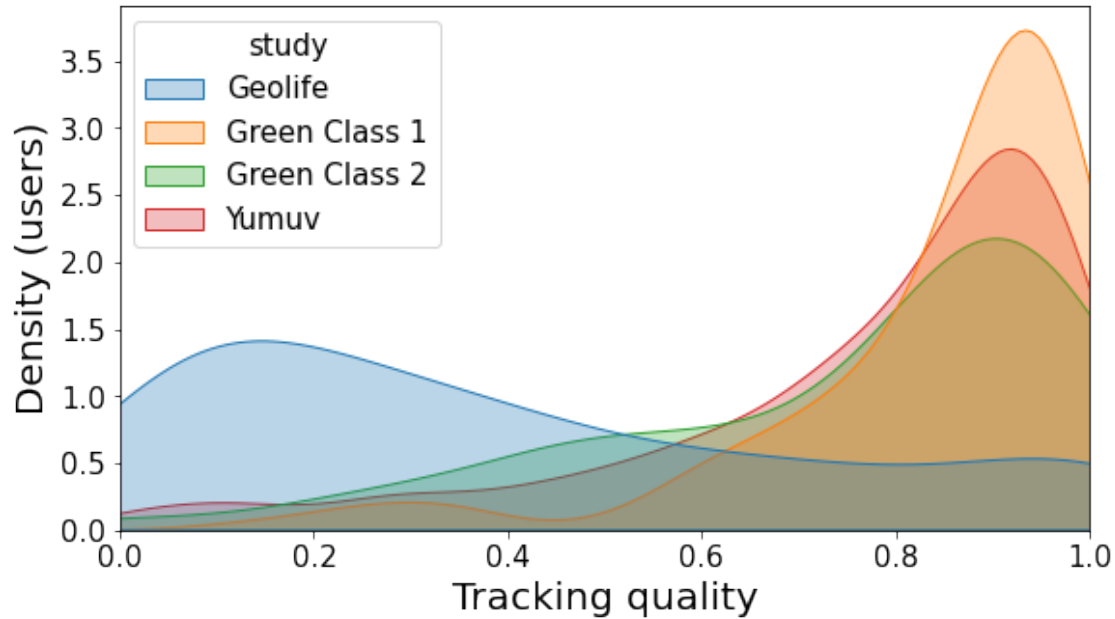

## 2.5 Modal split dataset comparison

We'll now show how trackintel can be used to analyze the modal split and compare it between different studies using the trackintel function `calculate_modal_split`. The datasets GC1, GC2 & yumuv have mode labels available while geolife does not feature mode labels for all triplegs. We therefore use the trackintel function `predict_transport_mode` to create labels.

Another preprocessing step is required because all studies use different mode labels. All of them will be matched to the three categories `fast`, `motorized` and `slow`

```
[96]: # Fill transport mode for geolife
is_geolife = triplegs["study"] == "Geolife"
triplegs.loc[is_geolife, "mode"] = predict_transport_mode(triplegs[is_geolife])
```

```
[97]: # we need to map the mode labels from GC1, GC2 & Yumuv to the ones from geolife
mode_to_category = {
    "Mode::Airplane": "fast",
    "Mode::Train": "fast",
    "airplane": "fast",
    "fast_mobility": "fast",
    "fast": "fast",
    "car": "motorized",
    "Mode::Boat": "slow",
    "Mode::Bus": "motorized",
    "Mode::Car": "motorized",
    "Mode::Coach": "motorized",
    "Mode::Ecar": "motorized",
}
```

```

    "Mode::Tram": "motorized",
    "bus": "motorized",
    "coach": "motorized",
    "ecar": "motorized",
    "motorbike": "motorized",
    "tram": "motorized",
    "motorized_mobility": "motorized",
    "motorized": "motorized",
    "Mode::Bicycle": "slow",
    "Mode::Ebicycle": "slow",
    "Mode::Walk": "slow",
    "bicycle": "slow",
    "boat": "slow",
    "ebicycle": "slow",
    "kick_scooter": "slow",
    "ski": "slow",
    "train": "fast",
    "walk": "slow",
    "slow": "slow",
    "slow_mobility": "slow",
}

# change mode labels with the above mapping
triplegs["mode"] = triplegs["mode"].map(mode_to_category)
triplegs.dropna(subset=["mode"], inplace=True)
triplegs["mode"].unique()

```

```
[97]: array(['slow', 'motorized', 'fast'], dtype=object)
```

### 2.5.1 Get modal split by count, duration and distance

```

[98]: # count
modal_split_count = triplegs.groupby("study").apply(
    calculate_modal_split, metric="count", norm=True
)
modal_split_count = modal_split_count.droplevel(1)
modal_split_count

```

```

[98]: mode          fast  motorized    slow
study
Geolife          0.009270  0.409317  0.581413
Green Class 1    0.128245  0.377709  0.494046
Green Class 2    0.138213  0.257223  0.604564
Yumuv            0.067272  0.259749  0.672979

```

```

[99]: # duration
modal_split_duration = triplegs.groupby("study").apply(

```

```

        calculate_modal_split, metric="duration", norm=True
    )
    modal_split_duration = modal_split_duration.droplevel(1)
    modal_split_duration

```

```

[99]: mode                fast  motorized      slow
      study
Geolife          0.025935   0.467538   0.506527
Green Class 1    0.281664   0.474181   0.244155
Green Class 2    0.285285   0.320476   0.394239
Yumuv            0.144173   0.358140   0.497688

```

```

[100]: # distance
modal_split_distance = triplegs.groupby("study").apply(
    calculate_modal_split, metric="distance", norm=True
)
modal_split_distance = modal_split_distance.droplevel(1)
modal_split_distance

```

```

[100]: mode                fast  motorized      slow
      study
Geolife          0.627340   0.297629   0.075030
Green Class 1    0.539562   0.421444   0.038994
Green Class 2    0.701996   0.230656   0.067348
Yumuv            0.451134   0.443738   0.105128

```

## 2.5.2 Plotting

```

[245]: colors = ["#1D2F6F", "#8390FA", "#6EAF46", "#FAC748"]
color = dict(zip(
    ["fast", "motorized", "slow"], ["#1D2F6F", "#8390FA", "#6EAF46"]
))

def plot_modal_split_comparison(split_type, modal_split_df):

    fig, ax = plt.subplots(figsize=(8, 5))
    modal_split_df.plot.bar(stacked=True, color=color, ax=ax)
    fs = 16
    legend_loc = "lower left" if split_type=="distance" else "upper right"
    plt.legend(loc=legend_loc, framealpha=1, fontsize=fs)
    plt.xlabel("Dataset", fontsize=fs+2)
    plt.ylabel(f"Modal split ({split_type})", fontsize=fs+2)
    plt.xticks(fontsize=fs, rotation=0)
    plt.tight_layout()
    plt.savefig(os.path.join(
        out_path, f"modal_split_all_{split_type}.pdf"
    ))

```

```
), bbox_inches="tight")  
plt.show()
```

```
[246]: # create plot for all modal split types  
for split_type, modal_split_df in zip(  
    ["count", "duration", "distance"],  
    [modal_split_count, modal_split_duration, modal_split_distance],  
):  
    plot_modal_split_comparison(split_type, modal_split_df)
```

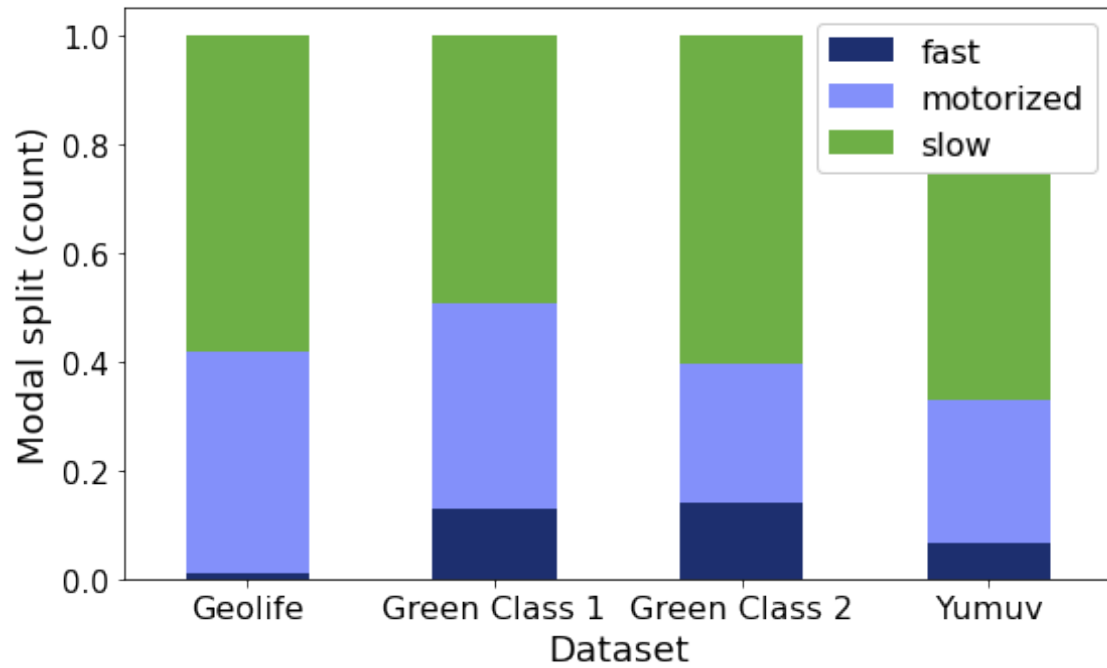

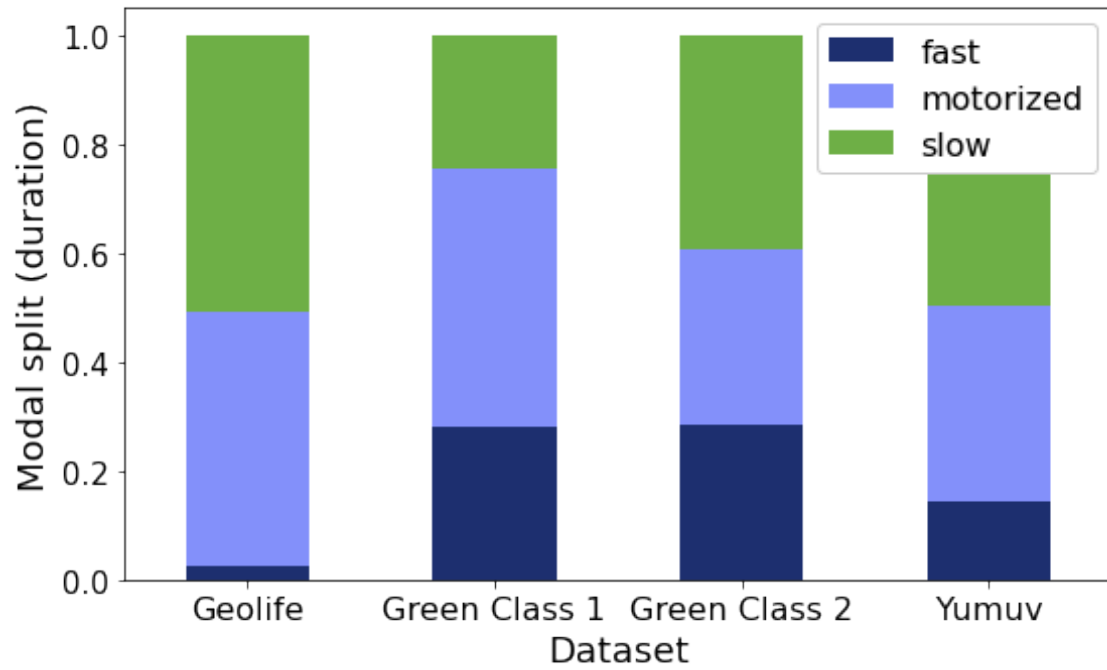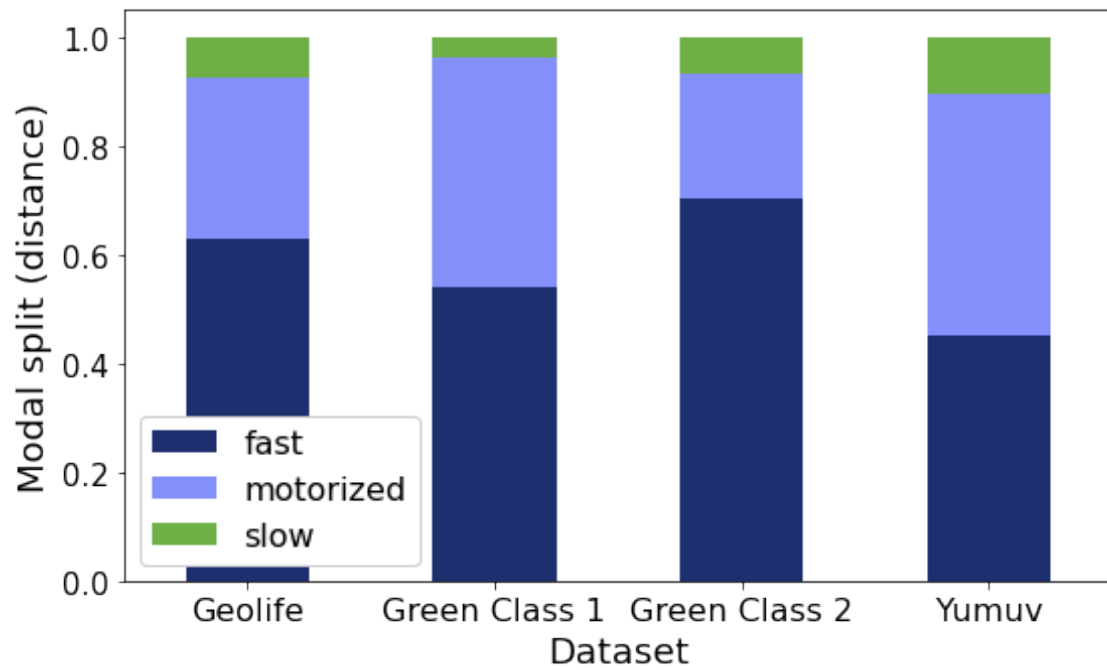

## 2.6 Home / Work labeling

In this section trackintel is used to analyze the activity patterns of participants of the different datasets. In the Green Class 1&2 datasets, the activity labels were provided by the participants. To analyze all datasets we'll first infer the major activity labels in the Geolife and yumuv dataset using the trackintel method `location_identifier`.

### 2.6.1 Compute staypoint purpose for Geolife and Yumuv

```
[106]: yumuv_geolife_flag = staypoints["study"].isin(["Geolife", "Yumuv"])

        staypoints.loc[yumuv_geolife_flag, "purpose"] = ti.analysis.location_identifier(
            staypoints.loc[yumuv_geolife_flag], pre_filter=False
        )["purpose"]
```

### 2.6.2 Select work or home for analysis

In the following we will analyze the distribution of home or work activity staypoints over time. To chose the analysis, the variable `home_work_variable` is either set to "home" or "work"

```
[327]: # Chose to analyze "home" or "work" activity staypoints
        home_work_variable = "home"
```

### 2.6.3 Data preparation for plotting

```
[328]: # Use either the home staypoints or the work staypoints
        if home_work_variable == "home":
            sp_study = staypoints[staypoints["purpose"] == "home"].copy()
        elif home_work_variable == "work":
            sp_study = staypoints[staypoints["purpose"] == "work"].copy()
```

```
[329]: # convert timestamp columns
        sp_study.loc[:, "started_at"] = sp_study.loc[
            :, "started_at"].dt.tz_convert("Europe/Paris")
        sp_study.loc[:, "finished_at"] = sp_study.loc[
            :, "finished_at"].dt.tz_convert("Europe/Paris")
```

### 2.6.4 Data transformation

To create a nice plot, we calculate the density of home or work staypoints in every minute bin. For this the staypoints are resampled with a minute resolution and then later aggregated again.

```
[330]: # chop up durations to minute-by-minute time series
        sp_study = sp_study[["started_at", "finished_at", "study"]]

        # create a column that contains date ranges with minute resolution
        sp_study["date"] = sp_study.apply(
            lambda x: pd.date_range(
                x["started_at"], x["finished_at"], freq="min")
```



```

    , axis=1
)
sp_study_expl = sp_study.explode("date", ignore_index=True).drop(
    columns=["started_at", "finished_at"]
)

```

```

[331]: # create hour & minute attributes used for aggregation later.
# Get Geolife in local time zone
geolife_flag = sp_study_expl["study"] == "Geolife"
sp_study_expl.loc[~geolife_flag, "hour"] = sp_study_expl.loc[
    ~geolife_flag, "date"
].dt.hour
sp_study_expl.loc[geolife_flag, "hour"] = sp_study_expl.loc[
    geolife_flag, "date"
].dt.tz_convert("Asia/Shanghai").dt.hour
sp_study_expl["minute"] = sp_study_expl.date.dt.minute
sp_study_expl["day"] = sp_study_expl.date.dt.date
sp_study_expl.head(3)

```

```

[331]:

```

|   | study   | date                      | hour | minute | day        |
|---|---------|---------------------------|------|--------|------------|
| 0 | Geolife | 2009-03-30 08:20:40+02:00 | 14.0 | 20     | 2009-03-30 |
| 1 | Geolife | 2009-03-30 08:21:40+02:00 | 14.0 | 21     | 2009-03-30 |
| 2 | Geolife | 2009-03-30 08:22:40+02:00 | 14.0 | 22     | 2009-03-30 |

```

[332]: # aggregate by hour and minute of every day for every study
count_by_minute = pd.DataFrame(sp_study_expl.groupby(
    ["study", "day", "hour", "minute"]
).size()).rename({0: "nr_home_sp"}, axis=1)

```

```

[333]: count_by_minute.reset_index(inplace=True)
count_by_minute["minute_of_day"] = count_by_minute[
    "hour"] * 60 + count_by_minute["minute"]
count_by_minute.head(3)

```

```

[333]:

```

|   | study   | minute_of_day | users_at_home |
|---|---------|---------------|---------------|
| 0 | Geolife | 0.0           | 0.520938      |
| 1 | Geolife | 1.0           | 0.520791      |
| 2 | Geolife | 2.0           | 0.520882      |

```

[334]: count_by_minute.tail(3)

```

```

[334]:

```

|      | study | minute_of_day | users_at_home |
|------|-------|---------------|---------------|
| 5757 | Yumuv | 1437.0        | 0.676193      |
| 5758 | Yumuv | 1438.0        | 0.676623      |
| 5759 | Yumuv | 1439.0        | 0.677077      |

### 2.6.5 Normalize: Fraction of users at home/work for each minute

```
[335]: # Get the active number of users per day
active_users_per_day = staypoints.set_index("started_at").groupby(
    ["study", "user_id", pd.Grouper(freq="D")]
).size().reset_index()
active_users_per_day["day"] = active_users_per_day["started_at"].dt.date
active_users_per_day = active_users_per_day.groupby(
    ["study", "day"]
).size().reset_index().rename({0: "active_users"}, axis=1)
active_users_per_day.head(3)
```

```
[335]:
```

|   | study   | day        | active_users |
|---|---------|------------|--------------|
| 0 | Geolife | 2007-04-12 | 3            |
| 1 | Geolife | 2007-04-13 | 4            |
| 2 | Geolife | 2007-04-14 | 3            |

```
[336]: count_by_minute = count_by_minute.merge(
    active_users_per_day, left_on=["study", "day"],
    right_on=["study", "day"]
)
```

```
[337]: # compute the number of users at home per day
count_by_minute["users_at_home"] = count_by_minute[
    "nr_home_sp" ] / count_by_minute["active_users"]
```

```
[338]: # Aggregate over the days to get the average fraction of users at hoe
count_by_minute = count_by_minute.groupby(
    ["study", "minute_of_day"]
).agg({"users_at_home": "mean"}).reset_index()
```

### 2.6.6 Plotting

```
[339]: # reshape and normalize so that we can plot easily
count_by_minute_pivot = count_by_minute.pivot_table(
    columns="study", index="minute_of_day", values="users_at_home"
)
count_by_minute_pivot.head(3)
```

```
[339]:
```

| study         | Geolife  | Green Class 1 | Green Class 2 | Yumuv    |
|---------------|----------|---------------|---------------|----------|
| minute_of_day |          |               |               |          |
| 0.0           | 0.520938 | 0.687393      | 0.702919      | 0.681459 |
| 1.0           | 0.520791 | 0.687979      | 0.702329      | 0.681473 |
| 2.0           | 0.520882 | 0.688507      | 0.702768      | 0.681858 |

```
[340]: count_by_minute_pivot.plot()
plt.xticks(
    np.arange(0, len(count_by_minute_pivot.index), 120), np.arange(0, 24, 2)
)
plt.legend(loc="lower left")
plt.ylabel(f"Density of {home_work_variable} staypoint duration")
plt.xlabel("Hour of the day")
plt.savefig(os.path.join(
    out_path, f"plot_activity_distribution_{home_work_variable}.pdf"
))
plt.show()
```

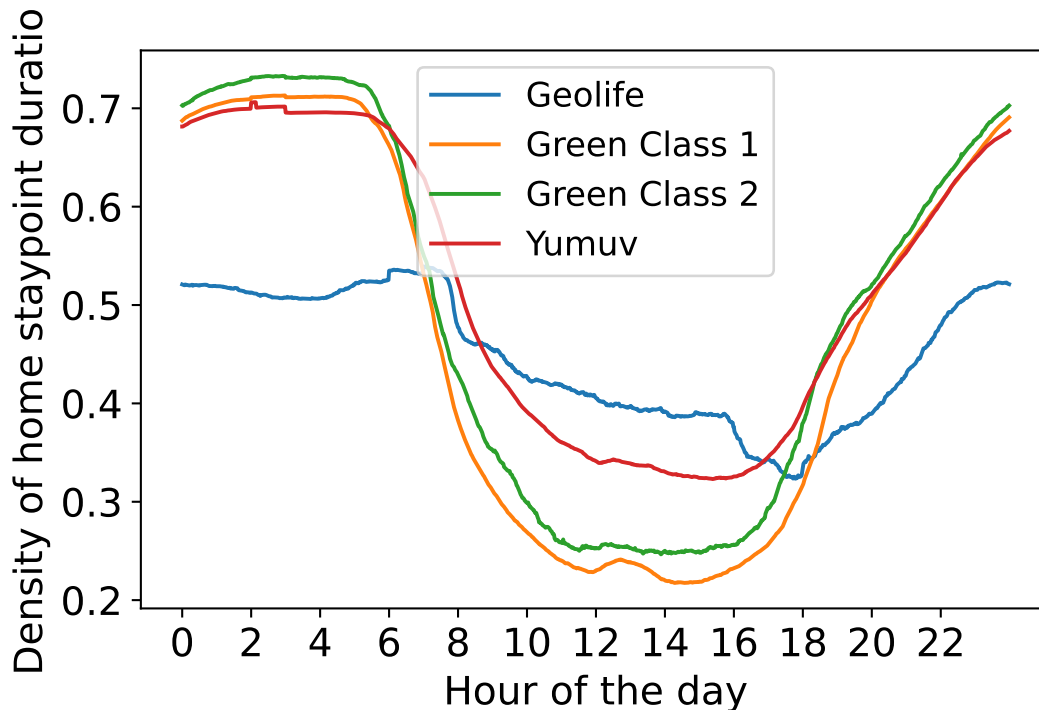

```
[341]: def plot_work_home_labels(home_work_variable, count_by_minute_pivot, fs=15):
fig, ax = plt.subplots(figsize=(12, 4))
home_slots = count_by_minute_pivot.values.transpose()
plt.imshow(home_slots, aspect=100)
for i in range(4):
    plt.plot([0, home_slots.shape[1]], [i + 0.5, i + 0.5], c="black", lw=1)
plt.xlim(0, 24)
plt.yticks(np.arange(4), count_by_minute_pivot.columns, fontsize=fs)
plt.xlabel("Hour of the day", fontsize=fs)
ax.xaxis.tick_top()
ax.xaxis.tickpad = -2
```

```

ax.xaxis.set_label_position("top")
plt.xticks(
    np.arange(0, len(count_by_minute_pivot.index), 120), np.arange(0, 24, 2),
    fontsize=fs
)
cbar = plt.colorbar(orientation="horizontal", ax=ax, aspect=16)
cbar.set_label(f"Average fraction of users at {home_work_variable}",
               fontsize=fs)
cbar.ax.tick_params(labelsize=fs)
plt.tight_layout()
plt.savefig(
    os.path.join(
        out_path, f"imshow_act_distribution_{home_work_variable}.pdf"
    ),
    bbox_inches="tight",
)
plt.title(f"Distribution of {home_work_variable} staypoints", fontsize=fs)
plt.show()

```

```

[342]: # Execute all cells from this section with home_work_variable="home"
plot_work_home_labels("home", count_by_minute_pivot)

```

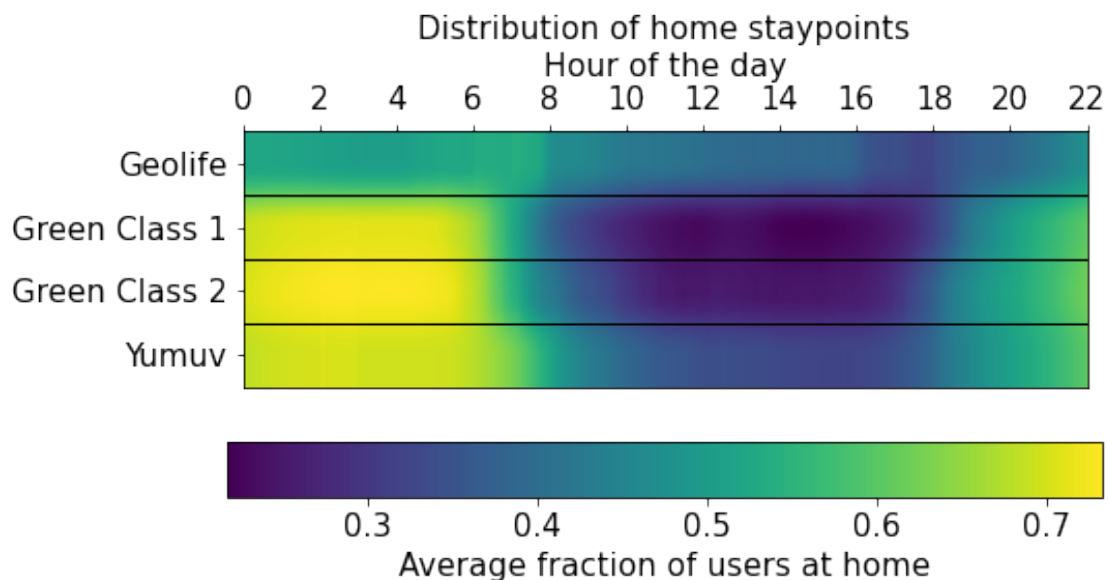

```

[326]: # Execute all cells from this section with home_work_variable="work"
plot_work_home_labels("work", count_by_minute_pivot)

```

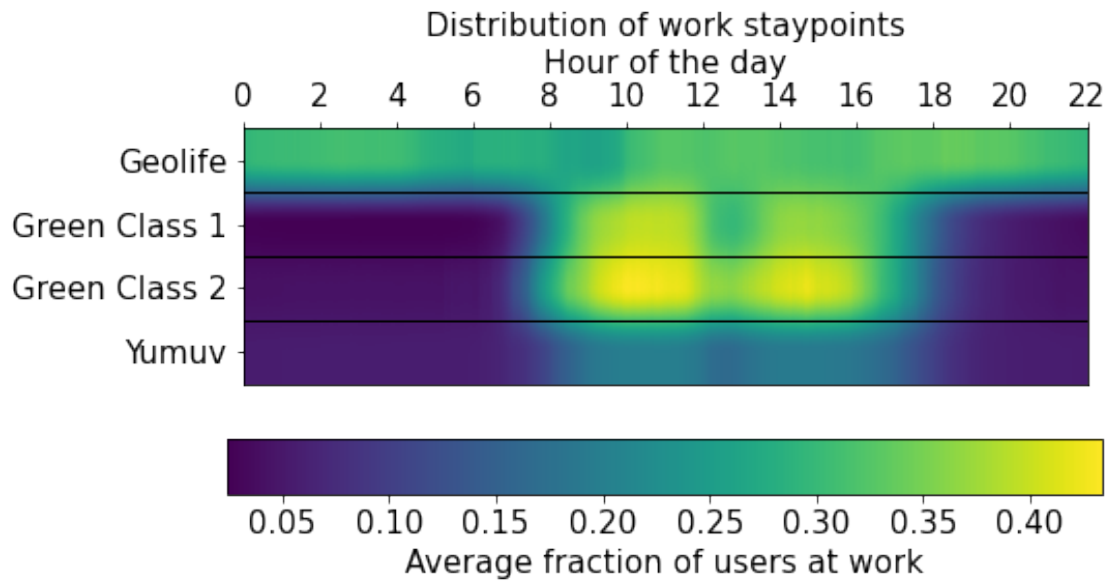

## 2.7 Visualization for individual users - Tracking data

Trackintel can also be used to visualize tracking data of individual users

### 2.7.1 Data collection

```
[275]: x_min = 116.2
x_max = 116.5
y_min = 39.8
y_max = 40.1
sw = Point(x_min, y_min)
se = Point(x_max, y_min)
ne = Point(x_max, y_max)
nw = Point(x_min, y_max)

study_area = gpd.GeoDataFrame(
    columns=["geometry"],
    data=[Polygon([sw, se, ne, nw])],
    geometry="geometry",
    crs="EPSG:4326",
)
```

```
[276]: # Load Geolife data of one user
tpls_vis = triplegs[triplegs["user_id"] == "51"].copy()
tpls_vis = ti.preprocessing.filter.spatial_filter(
    tpls_vis, study_area, method="within"
)
```

```
[277]: # Get staypoints as well for this user
sp_vis = staypoints[staypoints["user_id"] == "51"].copy()
sp_vis = ti.preprocessing.filter.spatial_filter(
    sp_vis, study_area, method="within"
)
```

```
[278]: # Get positionfixes for this user -
# using the pfs obtained with read_geolife function (see top of notebook)
pfs_vis = pfs_geolife[pfs_geolife["user_id"] == 51]
pfs_vis = ti.preprocessing.filter.spatial_filter(
    pfs_vis, study_area, method="within"
)
```

## 2.7.2 Plot all tracking data

```
[279]: ti.visualization.plot_triplegs(
    tpls_vis,
    staypoints=sp_vis,
    plot_osm=True,
    positionfixes=pfs_vis,
    staypoints_radius=150,
    out_filename=os.path.join(out_path, "geolife_tpls_sp_pfs"),
)
Image(filename=os.path.join(
    out_path, "geolife_tpls_sp_pfs.png"
), width=600, height=600)
```

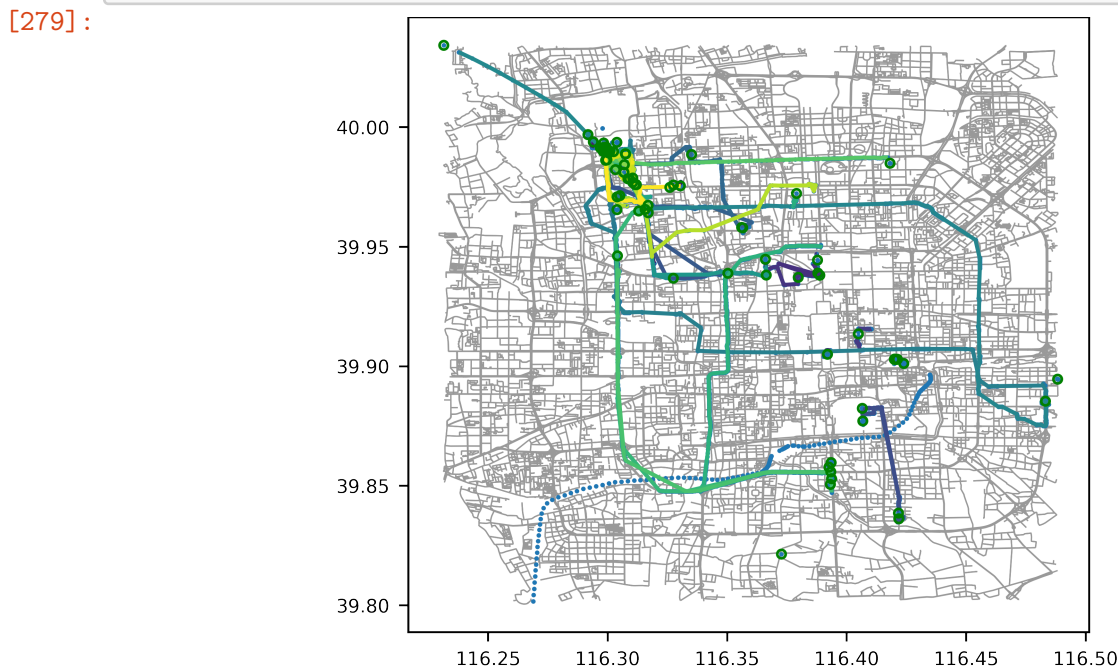

### 2.7.3 Plot only positionfixes

```
[280]: ti.visualization.plot_positionfixes(  
        pfs_vis, plot_osm=True, out_filename=os.path.join(out_path, "geolife_pfs")  
    )  
Image(  
    filename=os.path.join(out_path, "geolife_pfs.png"), width=500, height=500  
)
```

[280]:

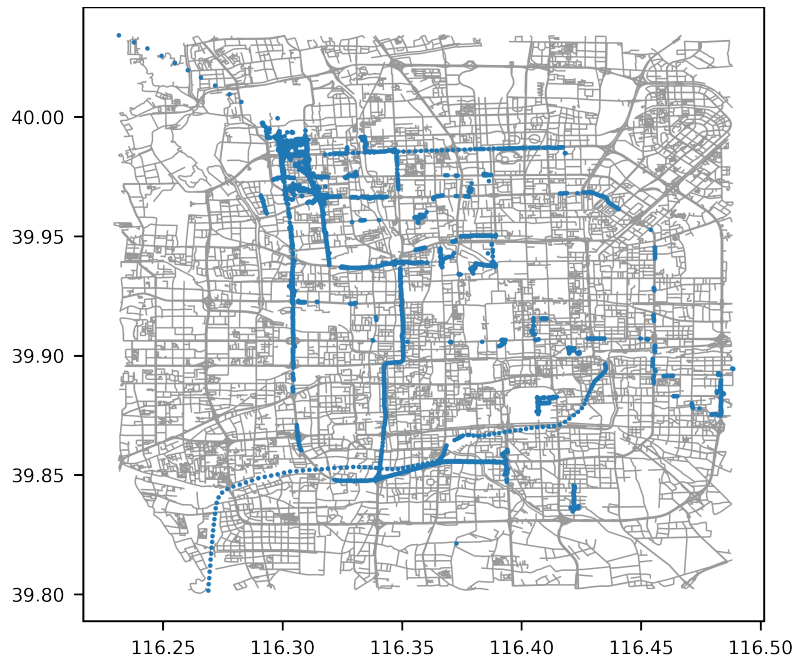

### 2.7.4 Plot staypoints with positionfixes

```
[281]: ti.visualization.plot_staypoints(  
        sp_vis,  
        positionfixes=pfs_vis,  
        plot_osm=True,  
        radius=150,  
        out_filename=os.path.join(out_path, "geolife_sp_pfs"),  
    )  
Image(filename=os.path.join(  
    out_path, "geolife_sp_pfs.png"  
), width=500, height=500)
```

[281]:

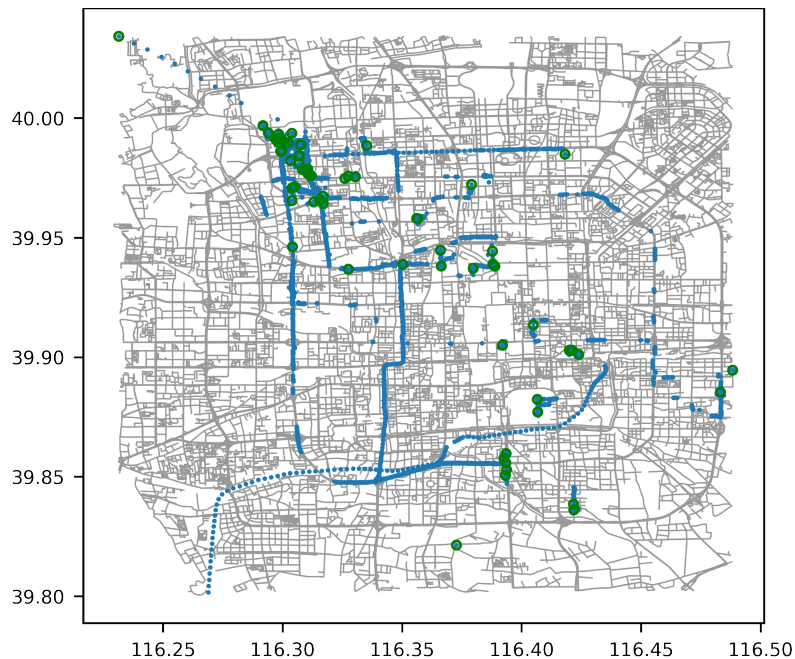

## 2.8 Visualization of individual users - Modal split

```
[282]: # Use one GC2 user for this visualization
tpls_vis = triplegs[
    triplegs["user_id"] == "c9aa08e2-1a5d-4d41-ae62-6110a9072b23"
].copy()
```

```
[283]: # rename to mode
tpls_vis["mode"] = tpls_vis["mode_detailed"]
```

### 2.8.1 Modal split - by count

```
[284]: # compute modal split
modal_split = calculate_modal_split(
    tpls_vis, freq="M", metric="count", per_user=False, norm=True
)
```

```
[285]: # order the transport modes for colour choices
column_order = [
    "Mode::Car",
    "Mode::Bicycle",
    "Mode::Walk",
    "Mode::Bus",
    "Mode::Train",
    "Mode::Ecar",
    "Mode::Ebicycle",
]
```



```

    "Mode::Airplane",
]
modal_split = modal_split[column_order]

```

```

[286]: fig, ax = plt.subplots(figsize=(5, 3))
ax = ti.visualization.modal_split.plot_modal_split(
    modal_split,
    date_fmt_x_axis="%b",
    y_label="Percentage of daily count",
    skip_xticks=0,
    n_col_legend=4,
    fig=fig,
    axis=ax,
    borderaxespad=2,
)
# fig.autofmt_xdate()
plt.savefig(os.path.join(out_path, "modal_split_count"))

```

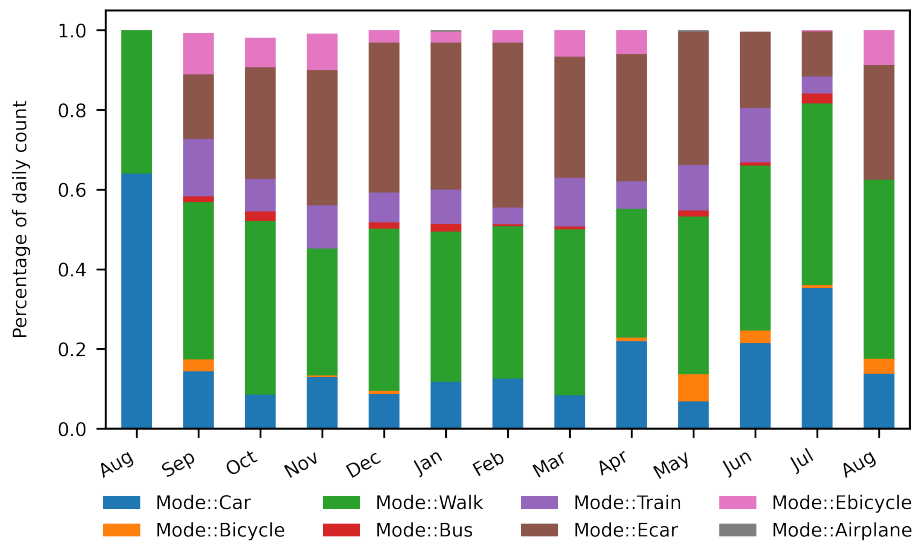

## 2.8.2 Modal split - by distance

```

[287]: modal_split = calculate_modal_split(
    tpls_vis, freq="M", metric="distance", per_user=False, norm=True
)
modal_split = modal_split[column_order]

```

```

[288]: fig, ax = plt.subplots(figsize=(5, 3))
ax = ti.visualization.modal_split.plot_modal_split(
    modal_split,

```

```

date_fmt_x_axis="%b",
y_label="Percentage of daily distance",
skip_xticks=0,
n_col_legend=4,
fig=fig,
axis=ax,
borderaxespad=2,
)
# fig.autofmt_xdate()
plt.savefig(os.path.join(out_path, "modal_split_distance"))

```

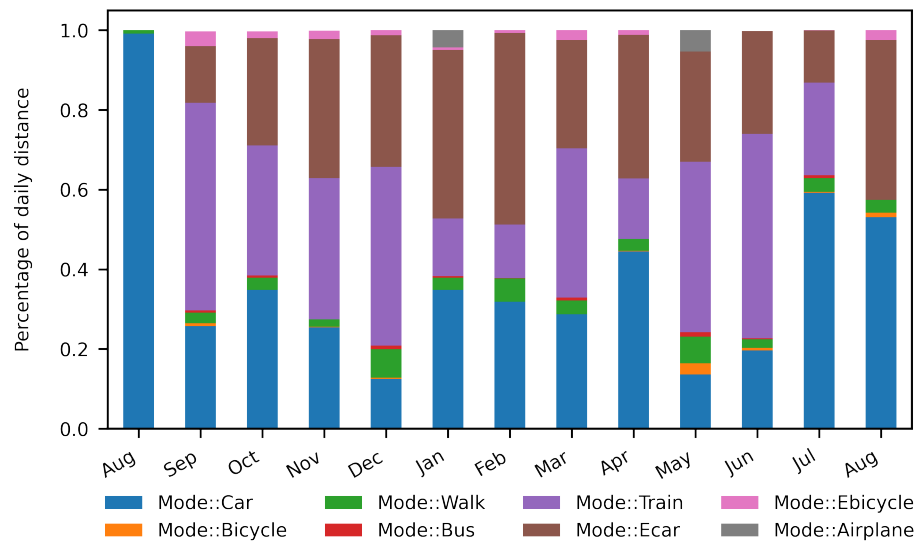

Supplement: Supplementary file 2 [file Trackintel_case_study.pdf]
